# Supplementary material for: Visual-Inertial Localization for Skid-Steering Robots with Kinematic Constraints
Source: arXiv:1911.05787 source file (2019-11-13)
Supplement: Supplementary file 1 [file appendix.tex]

\section*{Appendix}
The block matrix $\bm{\Phi}_A, \bm{\Phi}_B, \bm{\Phi}_C, \bm{\Phi}_D \in \mathbb{R}^{3 \times 3}$ appeared  in the error-state transition matrix can be computed by taking the derivative with respect to $\begin{bmatrix} X_v, Y_l, Y_r \end{bmatrix}^\top$ and $\begin{bmatrix} \alpha_l & \alpha_r \end{bmatrix}^\top$. 
%We omit some superscripts and subscripts for concise expression, which will not cause confusion.
%
\begin{align}
	\bm{\Phi}_A &\!=\!  {\Delta t} {}^{\mathbf{G}}_{{\mathbf O}_{k-1}} \hat{\mathbf{R}} \frac{\left( \hat{\alpha}_l o_{lm} - \hat{\alpha}_r o_{rm}\right)}{{\Delta \hat{Y}}^2}\! \begin{bmatrix}\begin{smallmatrix}
	0& \hat{Y}_r & - \hat{Y}_l\\
	{\Delta \hat{Y}} &- \hat{X}_v  & \hat{X}_v \\
	0 & 0& 0
	\end{smallmatrix} \! \end{bmatrix},
	\bm{\Phi}_B \!=\!  \Delta t  {}^{\mathbf{G}}_{{\mathbf O}_{k-1}}{\hat{\mathbf{R}} } \frac{1}{\Delta \hat{Y}}\begin{bmatrix}
	\begin{smallmatrix}
- \hat{Y}_r o_{lm}&  \hat{Y}_l o_{rm}\\
\hat{X}_v o_{lm}& -\hat{X}_v o_{rm}\\
0& 0
\end{smallmatrix} 
\end{bmatrix}
\end{align}
\begin{align}
\bm{\Phi}_C = \Delta t \cdot \frac{1}{{\Delta \hat{Y}}^2} \mathbf{J}_r  
\begin{bmatrix}\begin{smallmatrix}
0& 0& 0\\
0& 0& 0\\
0&  {\hat{\alpha}_l o_{lm}} - {\hat{\alpha}_r o_{rm}}&  -{\hat{\alpha}_l o_{lm}} + {\hat{\alpha}_r o_{rm}} \\
\end{smallmatrix}\end{bmatrix}
\end{align}
\begin{align}
\bm{\Phi}_D =  \Delta t \cdot \frac{1}{\Delta \hat{Y}} \mathbf{J}_r 
\begin{bmatrix}
0& 0\\
0& 0\\
- o_{lm}& o_{rm}
\end{bmatrix}
\end{align}
where $\mathbf{J}_r$ denotes the right Jacobian of ${}^{{\mathbf O}_{k-1}}\bm{\omega}_{zm} \Delta t$. If $\bm{\theta} = {\theta} \mathbf{a}\notag$, the following holds:
\begin{align}
\begin{matrix}
    	\mathbf{J}_r\left( \bm{\theta} \right) = \frac{\sin \theta}{\theta}\mathbf{I} + \left( 1- \frac{\sin \theta}{\theta} \right)\mathbf{a}\mathbf{a}^\top - \frac{1- \cos \theta}{\theta}\lfloor \mathbf{a} \rfloor
\end{matrix}
\end{align}
